# Supplementary material for: Exploring the Benefits of Teams in Multiagent Learning
Source: arXiv:2205.02328 source file (2023-07-31)
Supplement: Supplementary file 1 [file appendix_rogue.tex]

\subsection{Unreliable Agents}

\subsubsection{IPD Definition}

In the main text, we defined an unreliable agent in the IPD as defecting with probability $d$ at each timestep.
This design is chosen due to the emergence of an additional social dilemma when a teammate defects instead of acts randomly, explained below.

Assume that agents on any team $T_j$ are expected to cooperate with agents on $T_i$ if the agents in $T_i$ choose to cooperate with high frequency.
Similar to a Collective Risk Dilemma (CRD)~\cite{Merhej2021CooperationBI}, suppose if agents in $T_i$ collectively cooperate with $T_j$ with a frequency above an arbitrary threshold $\tau$, $C^{T_i}_{T_j} > \tau$, then agents in $T_j$ will mutually cooperate.
Although defecting on a cooperator yields the highest short-term utility, stable mutual cooperation leads to higher long-term reward in mixed-motive domains.
As a result, agents might want to cooperate with non-teammates to preserve a stable cooperative coalition.
Each agent in $T_i$ is responsible for $\frac{C^{T_i}_{T_j}}{|T_i|}$ of the collective cooperation, and each must cooperate at least $\frac{\tau}{|T_i|}$ to reach $\tau$.
Thus, an incompetent agent in the IPD as one which does not cooperate as much as its equal share, say $\frac{C^{T_i}_{T_j}}{|T_i|} - \epsilon$, where the agent chooses to defect with probability $d$ at each timestep.

\subsubsection{Team Size Mitigates Rogue Impact}

We now analyze the relationship between team size and the impact of rogue agents on other agents' perceived value of cooperating with that team.
Specifically, we show as $|T_i|$ increases, an agent's perceived value of cooperating with $T_i$ increases due to a decreased impact from the set of rogue agents $\mathbf{x}_{T_i}$. 
% The proof can be found in the appendix.

\begin{theorem}
The negative impact of $\mathbf{x}_{T_i}$ rogue agents on other agents' perceived value of cooperating with $T_i$ decreases as the size of the team increases ($|T_i| \rightarrow \infty$).
\label{thm:team_size_increase}
\end{theorem}

\begin{proof}
Let $n = |T_i|$ for improved readability.
Suppose agents on team $T_j$ will reciprocate cooperation if the frequency of cooperation from $T_i$ achieves some threshold $\tau$.
% , achieving a good reputation from the perspective of agents in $T_j$.
Let $\mathbf{x}_{T_i} \subset T_i$ be the set of rogue agents on team $T_i$ with $n - |\mathbf{x}_{T_i}|$ non-rogue agents who each cooperate with $T_j$ at least $\frac{\tau}{n}$.
Suppose rogue agents cooperate $\epsilon$ less than their non-rogue teammates, $\frac{\tau}{n} - \epsilon$.
For $C^{T_i}_{T_j} > \tau$, each non-rogue agent must now cooperate $\frac{\tau + |\mathbf{x}_{T_i}| \epsilon}{n}$.

Suppose $T_i$ increases to size $m$ but has the same set of rogue agents $\mathbf{x}_{T_i}$.
For the sake of contradiction, suppose non-rogue agents must now cooperate $\frac{\tau + |\mathbf{x}_{T_i}| \epsilon}{m} > \frac{\tau + |\mathbf{x}_{T_i}| \epsilon}{n}$ to ensure $C^{T_i}_{T_j} > \tau$.
The expression simplifies to $|\mathbf{x}_{T_i}| m \epsilon < |\mathbf{x}_{T_i}| n \epsilon$, or $m < n$.
Since we increased the size of $T_i$, we know $m > n$ must be true, a contradiction.
Thus, as the team size increases and the number of rogue agents is consistent, the extra effort required by each agent to achieve $\tau$ decreases.
\end{proof}

% Refer to the appendix for the proof of Theorem \ref{thm:team_size_increase}.

An important observation is the relationship between $|\mathbf{x}_{T_i}|$ and the amount rogue agents defect, $\epsilon$.
There may be a scenario where the set of non-rogue agents are unable to reach $\tau$, even if they always cooperate, possibly due to rogue agents with high degrees of defecting or making up the majority of $T_i$.
We calculate an upper bound on $|\mathbf{x}_{T_i}|$ and $\epsilon$ determined so the following constraint holds,
\[
|T_i| - |\mathbf{x}_{T_i}| (I - \frac{\tau}{|T_i|}) > |\mathbf{x}_{T_i}| \epsilon,\]
where $I$ is the expected number of interactions among agents.
Since the expected value of $I$ will be the same for all agents by Proposition \ref{thm:same_plays}, non-rogue agents must be able to cooperate enough to offset their rogue teammates, otherwise $C^{T_i}_{T_j} < \tau$ is unavoidable.
